# Supplementary material for: Local Coordination Modulates the Reflectivity of Liquefied Si-Ge Alloys
Source: arXiv:2310.17205 source file (2024-02-05)
Supplement: Supplementary file 1 [file Supplemental_Material.pdf]

## Supplemental Material Associated to: Local Coordination Modulates Reflectivity of Liquefied Si-Ge Alloys

Damiano Ricciarelli<sup>1\*</sup>, Ioannis Deretzis<sup>1</sup>, Gaetano Calogero<sup>1</sup>, Giuseppe Fisicaro<sup>1</sup>, and Antonino La Magna<sup>1\*</sup>

<sup>1</sup> National Research Council of Italy, Institute for Microelectronics and Microsystems (IMM-CNR), VIII Strada 5, 95121 Catania, Italy

E-mail: [damiano.ricciarelli@imm.cnr.it](mailto:damiano.ricciarelli@imm.cnr.it), [antonino.lamagna@imm.cnr.it](mailto:antonino.lamagna@imm.cnr.it)

### S1. Computational Methodology

Ab-initio molecular dynamics simulations on liquid Si, Si-Ge and Ge were performed following the approach proposed by Stich et al.<sup>1</sup> This approach, schematized in Figure S0, starts with a crystalline configuration and subjects it to extensive overheating well beyond the melting temperature to generate a profoundly disordered arrangement (pre-randomization). Subsequently, the system is thermally equilibrated at the melting point. Specifically, we pre-randomize for a total time of 1.0 ps, overheating at 6000 K and we ultimately thermalized the system for 4.5 ps. Only the last 3.5 ps are considered as production run, neglecting an equilibration time of 1.5 ps.

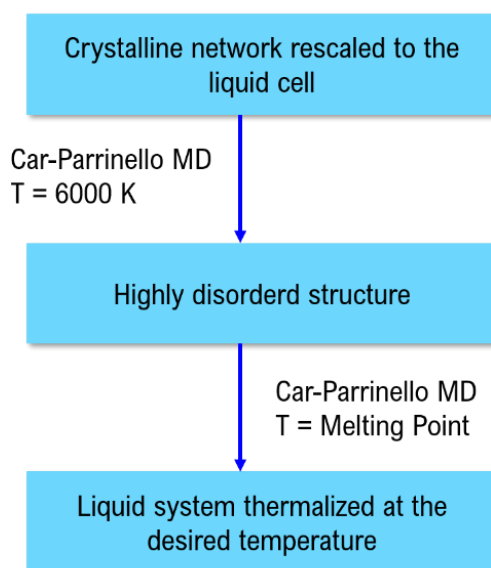

**Figure S0.** Schematics of the approach followed to model liquified Si, Si-Ge and Ge.

In our approach, where we employed 288 atoms fairly large 3x3x4 supercells, we utilized an NVT ensemble, incorporating cell parameters determined from experimental density at the melting point (Table S1)<sup>2</sup>. We employed the Car-Parrinello formulation of ab-initio molecular dynamics implemented in Quantum Espresso, performing integration over time with Verlet algorithm.<sup>3</sup> A time step of 0.0002 ps and a fictious electronic mass of 300 a.u are considered. Temperature is controlled by a Nose-Hoover thermostat employing a frequency of 5.0 GHz.<sup>1</sup>

**Table 1.** Parameters of liquids density's temperature dependent expression  $d = d_m + \alpha(T - T_m)$ .<sup>2</sup>

|                                                                                        |
|----------------------------------------------------------------------------------------|
| $d_{m, Si, l}; \alpha_{Si, l} = 2.5 gcm^{-3}; -3.5 \cdot 10^{-4} gcm^{-3} K^{-1}$      |
| $d_{m, SiGe, l}; \alpha_{SiGe, l} = 5.9 gcm^{-3}; -10.5 \cdot 10^{-4} gcm^{-3} K^{-1}$ |
| $d_{m, Ge, l}; \alpha_{Ge, l} = 5.6 gcm^{-3}; -5.9 \cdot 10^{-4} gcm^{-3} K^{-1}$      |

The ion-electron interaction is described by the Perdew-Burke-Ernzerhof (PBE) functional,<sup>4</sup> core electrons are mimicked by ultra-soft pseudopotentials,<sup>5</sup> dispersion contributions to the energy of the liquid are considered with D2 Van der Waals corrections,<sup>6</sup> the Brillouin zone is sampled at the k-point gamma. A cut-off on the plane waves basis set of 76 Ryd is applied, along with a cut-off on the electronic density of 239 Ryd.

Dielectric tensors are computed with the Random Phase Approximation (RPA) formalisms,<sup>7</sup> implemented in the same software. We made a post-processing of 10 random selected snapshots. To this aim density functional theory (DFT) parameters are slightly refined to obtain a better numerical accuracy: core electrons are described with Norm-Conserving Vanderbilt pseudopotentials,<sup>8</sup> electrons are smeared according to the Fermi-Dirac distribution at the melting temperature, the Brillouin zone is sampled with a uniform 2x2x2 grid.

The air-liquid interface reflectivity  $R$  is ultimately evaluated from RPA dielectric functions  $\epsilon$  (we here take a 3-dimensional average of the diagonal tensor), through real  $n$ , and complex  $k$  refractive indices.

$$n = \sqrt{\frac{Re(\epsilon) + \sqrt{Re(\epsilon)^2 + Im(\epsilon)^2}}{2}} \quad (1)$$

$$k = \frac{Im(\epsilon)}{2n} \quad (2)$$

$$R = \frac{(n-1)^2 + k^2}{(n+1)^2 + k^2} \quad (3)$$

Projected density of states, contribution of single particle states to the electron density and electron localization functions for further analysis are computed utilizing identical DFT parameters.

## Supplemental Structural and Data and Theory

The radial distribution function,  $g(r)$ , is calculated with (1),

$$g(r) = \frac{dn_r}{4\pi\rho r^2 dr} \quad (4)$$

where  $dn_r$  is the count for the specific bin of size  $dr$ ,  $r$  is the sphere radius and  $\rho$  is the liquid density.

The coordination number  $n(r)$  is calculated with

$$n(r) = 4\pi\rho \int_0^r g(r')r'^2 dr \quad (5)$$

The angular distribution function  $g(\theta)$  is calculated with

$$g(\theta) = \frac{1}{N_{\theta ij k}} \frac{dn_{\theta ij k}}{d\theta_{ij k}} \quad , \quad r_{ij}, r_{jk} < R_{cut} \quad (6)$$

where  $N_{angles}$  is the total number of considered  $\theta$  angles,  $dn_{\theta}$  is the count for the specific bin of size  $d\theta$ .

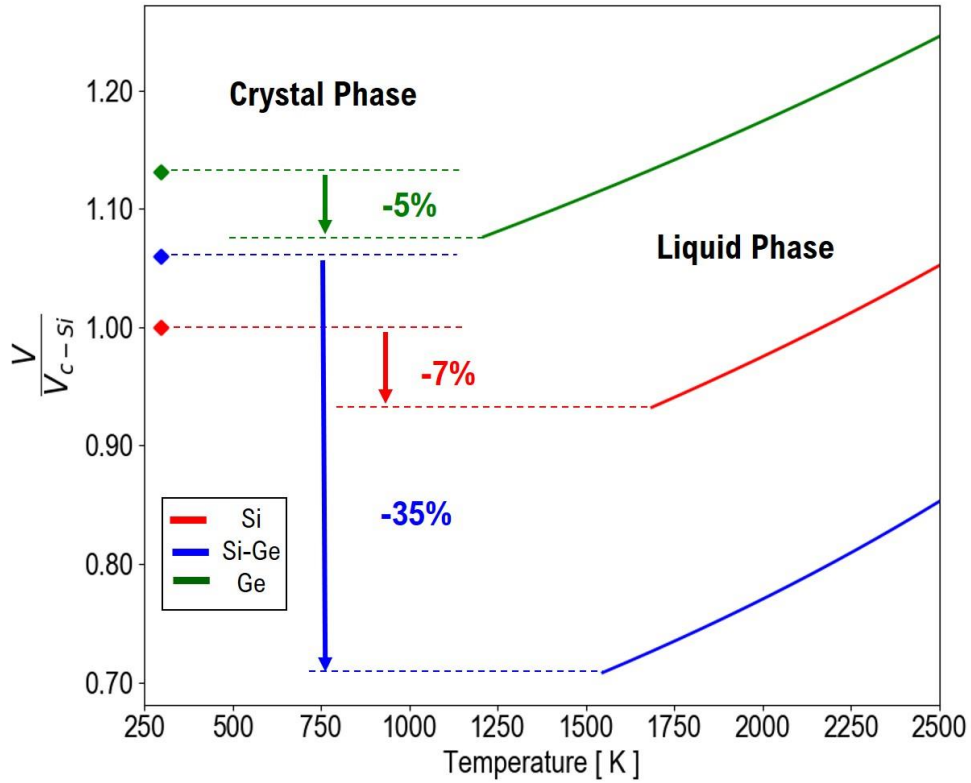

**Figure S1.** Volume shrinkage of Si, Si-Ge and Ge inherent to crystalline-liquid phase transition from ref. 2.

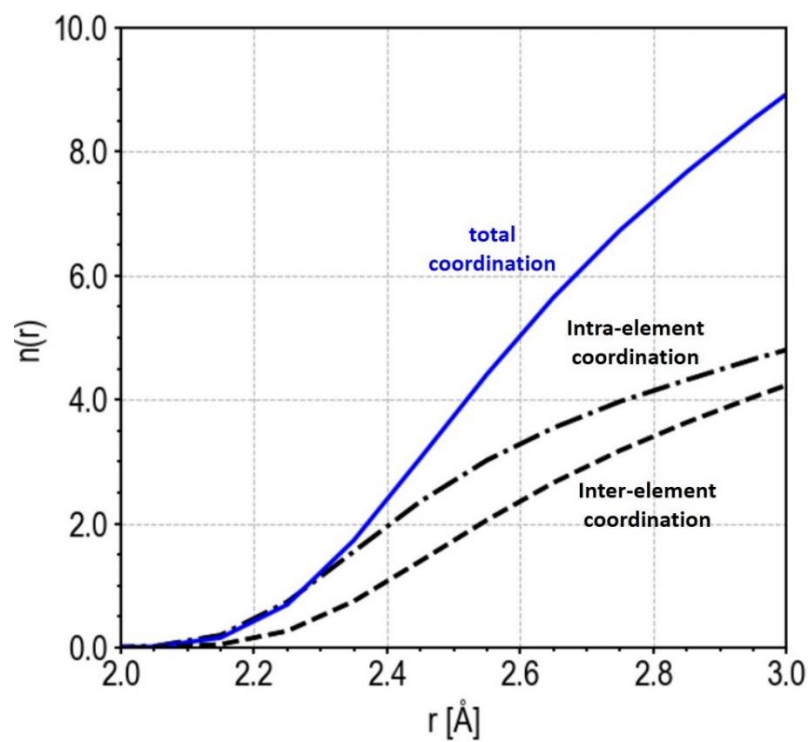

**Figure S2.** Decomposition of the  $n(r)$  function of Si-Ge into intra-element and inter-element contributions.

### Supplemental Electronic Structure Data

$$\overline{ELF}(z) = \frac{1}{L_x L_y} \int_0^{L_x} \int_0^{L_y} ELF(x, y, z) dx dy$$

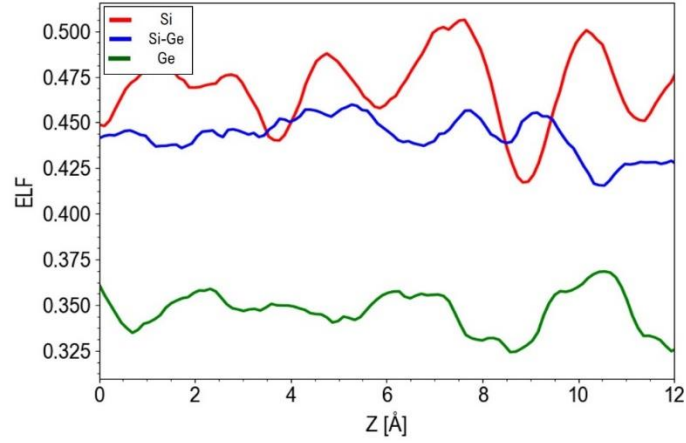

**Figure S3.** Planar average along the z-direction of the electron localization function (ELF) for liquid Si, Si-Ge and Ge at their respective melting temperature.

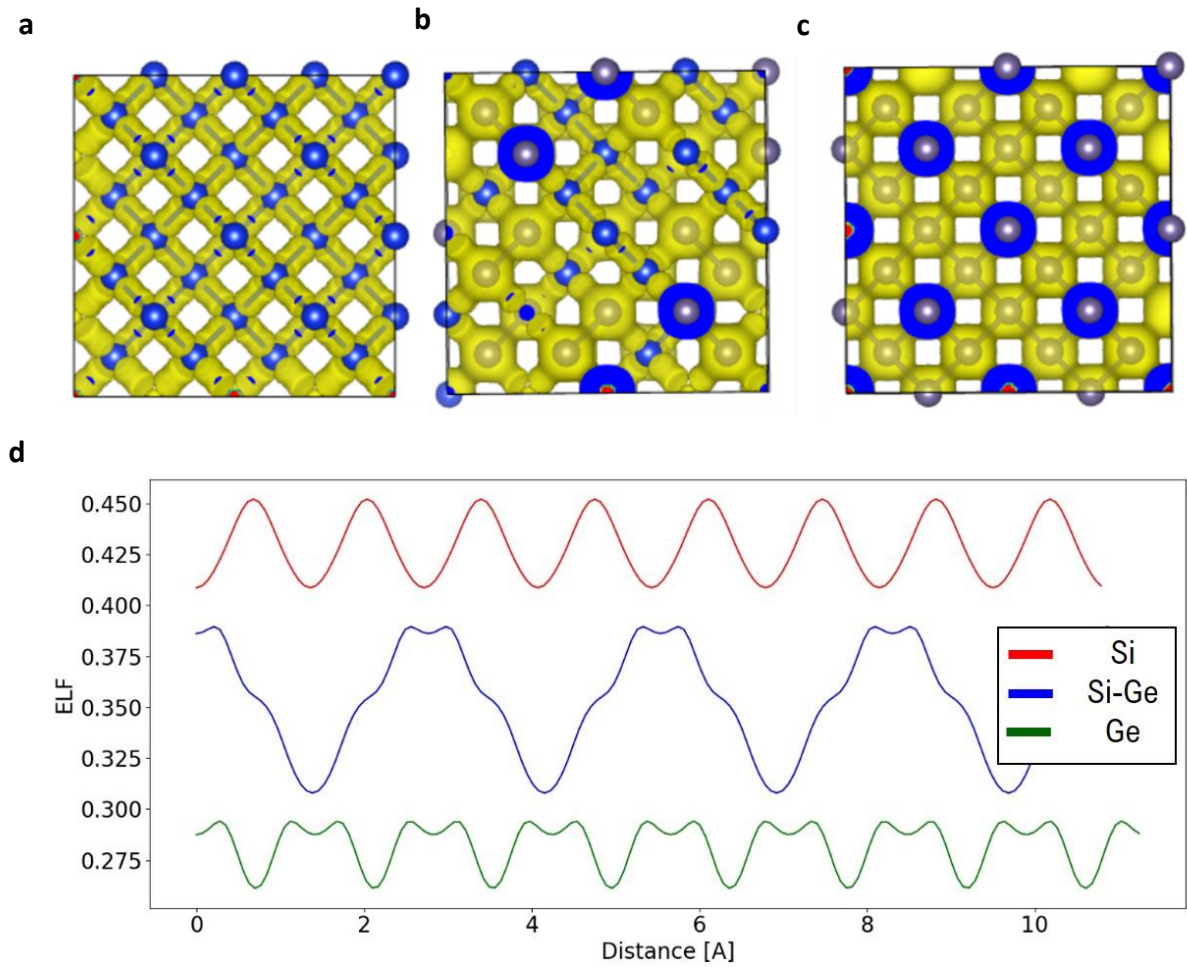

**Figure S4.** Electronic properties comparison for crystals: electron localization function (ELF) iso-value plots for crystalline (a) Si, (b) Si-Ge and (c) Ge, (d) planar average of ELF along the z-axis.

## Supplemental Optical Data

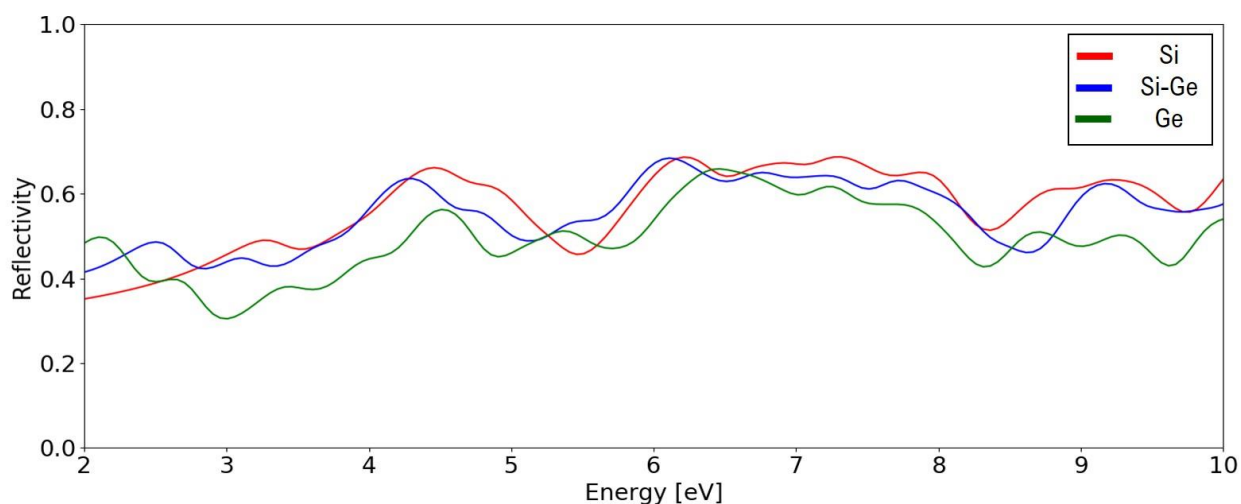

**Figure S5.** Reflectivity quantified from RPA\*. \*A rigid shift to the imaginary oscillator of amount  $[E_{\text{gap}}(\text{Exp.}) - E_{\text{gap}}(\text{PBE})]$  have been applied in the software to adjust the incorrect band gap predicted by the generalized gradient approximation.

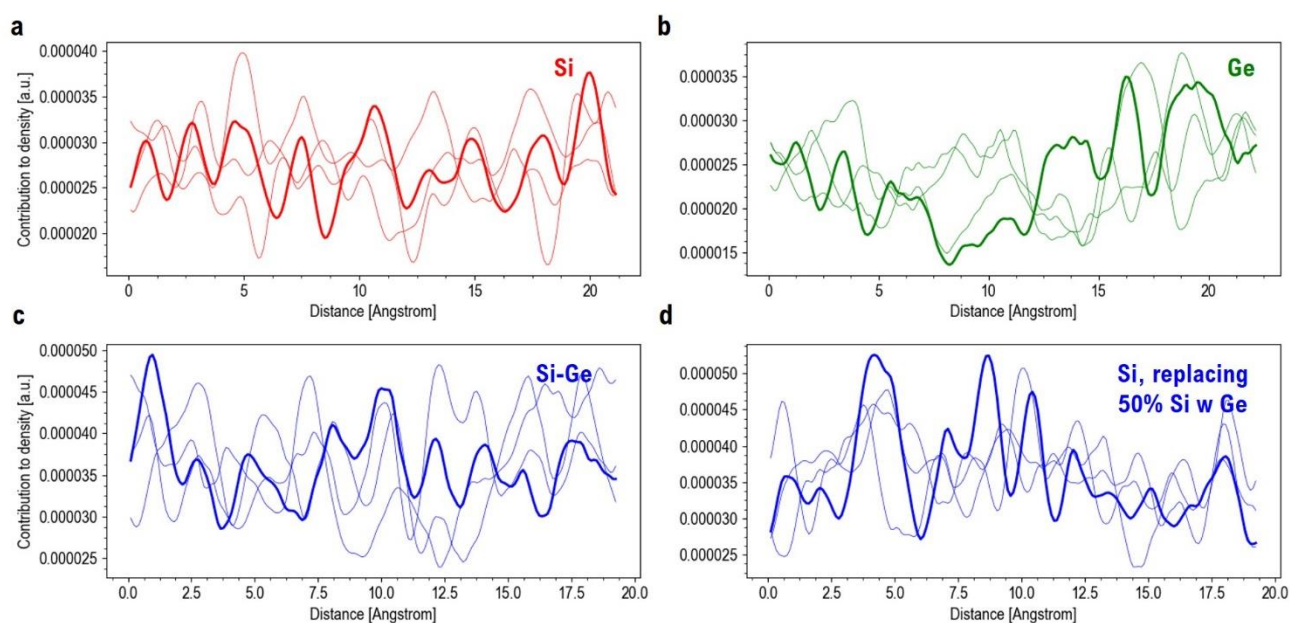

**Figure S5.** Planar average along the z-axis of contribution to the electron density for selected single-particle states following the structural correspondence: (a) Si, (b) Ge, (c) Si-Ge, (d) Si, replacing 50% Si w Ge at their melting temperature. The thicker line represents the planar average of the highest occupied single particle state, while the thinner lines represents lowest unoccupied, (lowest unoccupied + 20) and (lowest unoccupied + 40) single particle states.

### Additional data

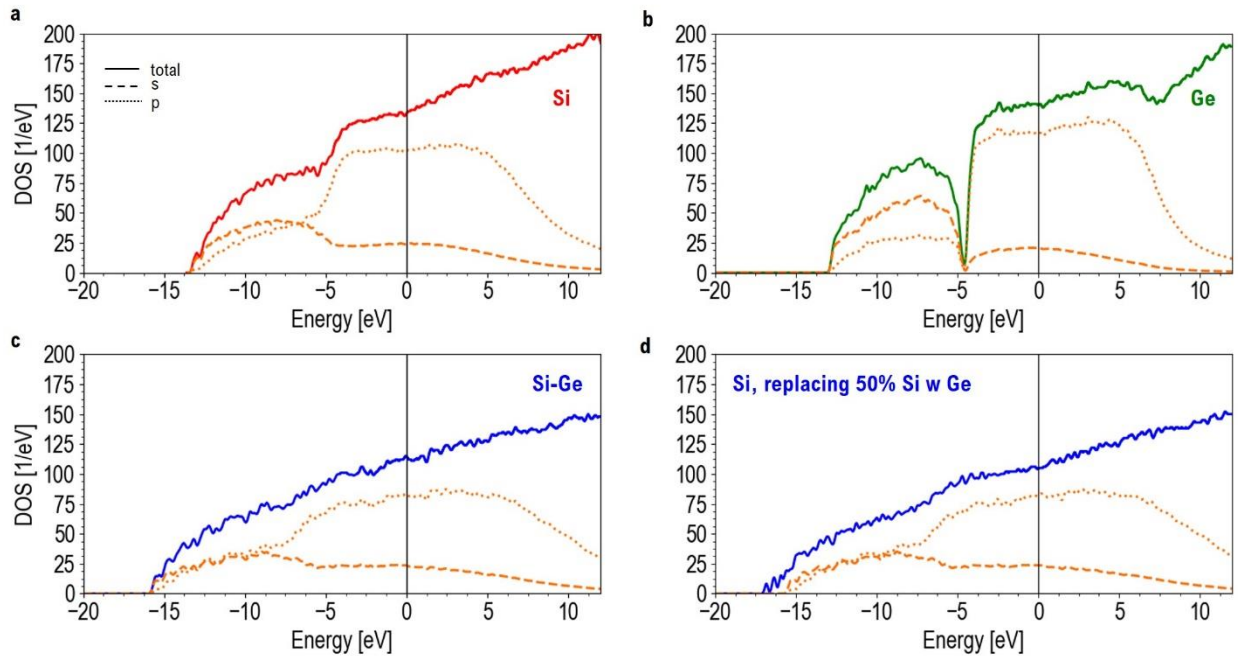

**Figure S7.** Density of states at melting temperature for (a) liquid Si, (b) liquid Ge, (c) liquid Si-Ge and (d) fictitious liquid Si-Ge computed upon Si structure.

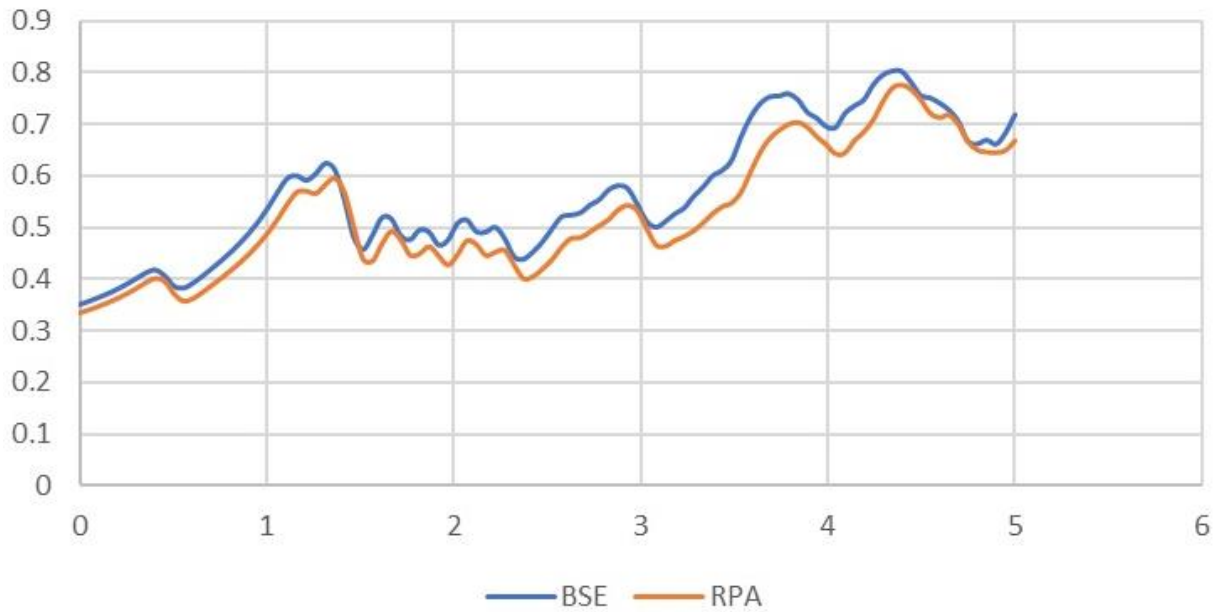

**Figure S8.** Comparison of reflectivities collected from Random Phase Approximation (RPA) and Bethe-Salpeter equation (BSE) formalisms for crystal Ge.

## References

1. I. Štich, R. Car, and M. Parrinello, Structural, bonding, dynamical, and electronic properties of liquid Si: An ab initio molecular-dynamics study, *Phys. Rev. B*, 1991, 44.9: 4262.
2. E. Ricci, S. Amore, D. Giuranno, R. Novakovic, A. Tuissi, N. Sobczak, R. Nowak, B. Korpala, and G. Bruzda, Surface tension and density of Si-Ge melts, *J. Chem. Phys.*, 2014, 140, 21
3. R. Car and M. Parrinello, Unified Approach for Molecular Dynamics and Density-Functional Theory, *Phys. Rev. Lett.*, 1985, 55, 2471
4. Perdew, J. P.; Burke, K.; Ernzerhof, M. Generalized Gradient Approximation Made Simple. *Phys. Rev. Lett.*, 1996, 77, 3865-3868
5. Vanderbilt, D. Soft self-consistent pseudopotentials in a generalized eigenvalue formalism, *Phys. Rev. B*, 1990, 41, 7892-7895
6. S. Grimme, Semiempirical GGA-type density functional constructed with a long-range dispersion correction. *J. Comput. Chem.*, 2006, 27: 1787-1799
7. N. E. Brener, Random-phase-approximation dielectric function for diamond, with local field effects included, *Phys. Rev. B*, 1975, 12, 1487
8. D. R. Hamann, Optimized norm-conserving Vanderbilt pseudopotentials, *Phys. Rev. B*, 2013, 88, 085117
9. D. Ricciarelli, G. Mannino, I. Deretzis, G. Calogero, G. Fisicaro, R. Daubriac, F. Cristiano, R. Demoulin, P. P. Michałowski, P. Acosta-Alba, and J.M. Hartmann, Impact of surface reflectivity on the ultra-fast laser melting of Si-Ge alloys, *Mater. Sci. Semicond. Proc.*, 2023, 165, 107635.
